# Supplementary material for: Initial data analysis of the national German transplantation registry with a focus on kidney transplantation
Source: arXiv:2601.02226 ancillary file (2026-03-27)
Supplement: Supplementary file 1 [file Additional_File_1.pdf]

# Supplementary Material

Lukas Klein Gunter Grieser Carl-Ludwig Fischer-Fröhlich
Axel Rahmel Henrik Stahl Andreas Wienke
Antje Jahn-Eimermacher

2026-01-05

## Table of contents


**1 Supplementary Table 1** **1**

**2 Supplementary Table 2** **3**

**3 Supplementary Information 1** **6**

**4 Supplementary Table 3** **6**

**5 Supplementary Table 4** **16**

**6 Supplementary Figure 1-3** **20**

**7 Supplementary Table 5** **23**

**8 Supplementary Table 6-8** **24**


## 1 Supplementary Table 1

This table lists the original names of the tables in the export and what entities they contain.

Table 1

| Table Name in Publication | Table Name in Export | Contains Recipients | Contains Transplan-tations | Contains Donors |
|---|---|---|---|---|
| T_Kidney_Waitlist | warteliste_niere | Yes | No | No |
| T_Recip_Immuno | empfaenger_immunologie | Yes | No | No |
| T_Recip_Urgency | empfaenger_dringlichkeit | Yes | No | No |
| T_Recip_Virology | empfaenger_virologie | Yes | No | No |
| T_Recipient | empfaenger | Yes | No | No |
| T_Kidney_Med | followup_niere_medikation | No | Yes | No |
| T_Postop_Exam | transplantation_postop_untersuchung | No | Yes | No |
| T_Kidney_Followup | followup_niere | Yes | Yes | No |
| T_Donor_PM | spender_postmortem | No | No | Yes |
| T_Donor_PM_Blood_Gas | spender_postmortem_labor_blutgase | No | No | Yes |
| T_Donor_PM_Blood_Type | spender_postmortem_labor_blutgruppe | No | No | Yes |
| T_Donor_PM_Chem | spender_postmortem_labor_klinische_chemie | No | No | Yes |
| T_Donor_PM_Diag | spender_postmortem_diagnosen | No | No | Yes |
| T_Donor_PM_Exams | spender_postmortem_untersuchungen | No | No | Yes |
| T_Donor_PM_HLA | spender_postmortem_labor_hla | No | No | Yes |
| T_Donor_PM_Med | spender_postmortem_medikation | No | No | Yes |
| T_Donor_PM_Micro | spender_postmortem_labor_mikrobiologie | No | No | Yes |
| T_Donor_PM_Monitor | spender_postmortem_monitoring | No | No | Yes |
| T_Donor_PM_Path | spender_postmortem_labor_pathologie | No | No | Yes |
| T_Donor_PM_Tox | spender_postmortem_labor_toxikologie | No | No | Yes |
| T_Donor_PM_Urine | spender_postmortem_labor_urin | No | No | Yes |
| T_Donor_PM_Virology | spender_postmortem_labor_virologie | No | No | Yes |
| T_Donor_PM_Crossmatch | spender_postmortem_labor_crossmatch | Yes | No | Yes |
| T_Kidney_Retrieval | organ_entnahme_niere | No | Yes | Yes |
| T_Transplantation | transplantation | Yes | Yes | Yes |

## 2 Supplementary Table 2

This table shows the original names of the columns in the export. For example `T_Transplantation.C_Destination` is the column `TBestimmungsortET` in `transplantation.csv`. The listed columns are relevant for the contents of this publication.

Table 2

| Table | Column Name in Export | Data providers | Column Name in Publication |
|---|---|---|---|
| T_Donor_PM_Blood_Type | SPostmLaborBlutGrUntersuchungsart | DSO | C_DiagType |
| T_Donor_PM_Chem | SPostmLaborKCKreatininWert | DSO, ET | C_Creatinine |
| T_Donor_PM_Crossmatch | SPostmLaborCrossmTXCET | DSO | C_TXC |
| T_Donor_PM_Crossmatch | SPostmLaborCrossmXMERG | DSO | C_XMERG |
| T_Donor_PM_Diag | SPostmDiagnosenKlassifikation | DSO | C_DiagClass |
| T_Donor_PM_Med | SPostmMedienDosisEinheit | DSO, ET | C_DosUnit |
| T_Donor_PM_Monitor | SPostmMonitHstillstandDauerWert | DSO, ET | C_ArrestDur |
| T_Donor_PM_Monitor | SPostmMonitDiureseZeitintervallWert | DSO, ET | C_DiuresisInterval |
| T_Donor_PM | SPostmAnamnVorerkrankungenDiabetesMellitus | DSO, ET | C_Diabetes |
| T_Donor_PM | SPostmAnamnVorerkrankungenHypertonie | DSO, ET | C_Hypertension |
| T_Donor_PM | SPostmAnamnMalignitaet | DSO, ET | C_Malign |
| T_Kidney_Followup | FNDate | ET, IQTIG | C_Date |
| T_Kidney_Followup | FNTodesdatum | IQTIG | C_DeathDate |
| T_Kidney_Followup | FNPatientVerstorben | IQTIG | C_DeathIndicator |
| T_Kidney_Followup | FNGraftversagenDate | IQTIG | C_FailureDate |
| T_Kidney_Followup | FNGraftversagen | IQTIG | C_FailureIndicator |
| T_Kidney_Followup | FNCenter | ET | C_FolUpCenter |
| T_Kidney_Followup | FNFollowUpArt | ET | C_FolUpType |
| T_Kidney_Retrieval | ONIschaemiezeitWarmErsteWert | DSO, ET | C_WarmIschemiaTime |
| T_Kidney_Waitlist | WNTransplantationenNAnzahl | ET | C_KidneyTXCount |
| T_Recip_Immuno | EImmDiagnostikZentrum | ET | C_DiagCenter |
| T_Recip_Immuno | EImmErgebnisTyp | ET | C_ResultType |
| T_Recip_Urgency | EDringlCode | ET | C_UrgeCode |
| T_Recipient | EBasisGeburtsdatum | ET, IQTIG | C_BirthDate |
| T_Recipient | EBasisGroesseWert | ET, IQTIG | C_BodyHeight |
| T_Recipient | EBasisGewichtEinheit | ET, IQTIG | C_BodyWeightUnit |

| | | | |
|---|---|---|---|
| T_Recipient | EBasisGewichtWert | ET, IQTIG | C_BodyWeight |
| T_Recipient | EBasisTodesdatum | ET | C_DeathDate |
| T_Transplantation | TBestimmungsort | ET | C_Destination |
| T_Transplantation | TPostOPOrganversagenDate | ET | C_FailureDate |
| T_Transplantation | TFollowUpZentrum | ET | C_FolUpCenter |
| T_Transplantation | TFollowUpLetztesDate | ET | C_LastDate |
| T_Transplantation | TOrgan | ET | C_Organ |
| T_Transplantation | TTransplantationszentrumRegistrierung | ET | C_RegCenter |
| T_Transplantation | TTransplantationszentrum | ET | C_TXCenter |
| T_Transplantation | TTxDate | ET, IQTIG | C_TXDate |

# 3 Supplementary Information 1

To construct our target population, we first joined the 78,666 recipients in `T_Recipient` table and transplantations reported by ET in `T_Transplantation` on the ET recipient identifier. This lead to 44629 recipients. Afer calculating the age at the time of the transplantation by calculating the difference between `T_Recipient.C_BirthDate` and `T_Transplantation.C_TXDate`, we filtered for recipients older then 18 years and who had both columns not missing. This lead to 41,984 recipients. To only keep kidney recipients, `T_Transplantation.C_Organ` had to be either "Left Kidney" or "Right Kidney". This lead to 24,760 recipients. To filter for first-time kdiney-only recipients, we filtered recipients who had multiple observations reported by ET in `T_Transplantation`, which reduced the number of recipients to 24,054. Furthmore to filter recipients, who might have had kidney trasnplantations not listed in the TxReg data, the column `T_T_Kidney_Waitlist.C_KidneyTXCount` had to have a non-missing value equal or below 1. This lead to 21,283 recipients. Finally, to only include data from deceased donors, the donors for the transplantations had to have an entry in `T_Donor_PM`, leading to the final number of recipients 14,954.

# 4 Supplementary Table 3

This table shows the columns which were in clusters 3 and 4 of the flux analysis.

Table 3

| Cluster | Table | Column Prefix in Export | Influx | Outflux | Proportion of Missing Values |
|---|---|---|---|---|---|
| 3 | `T_Kidney_Med` | `FNImmunsuppression-DateET` | 0.000 | 1.000 | 0.00% |
| 3 | `T_Kidney_Med` | `FNImmunsuppression-IdTransplantations-NrET` | 0.000 | 1.000 | 0.00% |
| 3 | `T_Kidney_Med` | `FNImmunsuppression-NameET` | 0.000 | 1.000 | 0.00% |
| 3 | `T_Recip_Urgency` | `EDringlCodeET` | 0.000 | 1.000 | 0.00% |
| 3 | `T_Recip_Urgency` | `EDringlDateET` | 0.000 | 1.000 | 0.00% |
| 3 | `T_Recip_Urgency` | `EDringlId-EmpfaengerNrETET` | 0.000 | 1.000 | 0.00% |
| 3 | `T_Recip_Urgency` | `EDringlOrganET` | 0.000 | 1.000 | 0.00% |

| | | | | | |
|---|---|---|---|---|---|
| 3 | T_Postop_Exam | TPostOPUntersuchung-DateET | 0.000 | 1.000 | 0.00% |
| 3 | T_Postop_Exam | TPost-OPUntersuchungId-Transplantationsnummer-ETET | 0.000 | 1.000 | 0.00% |
| 3 | T_Postop_Exam | TPostOPUntersuchung-KreatininWertET | 0.001 | 0.819 | 0.10% |
| 3 | T_Recipient | EBasisBlutgrET | 0.000 | 1.000 | 0.00% |
| 3 | T_Recipient | EBasisGeburtsdatum-ET | 0.000 | 1.000 | 0.00% |
| 3 | T_Recipient | EBasisGeschlechtET | 0.000 | 1.000 | 0.00% |
| 3 | T_Recipient | EBasisGewicht-EinheitET | 0.000 | 1.000 | 0.00% |
| 3 | T_Recipient | EBasisGewichtWert-ET | 0.000 | 1.000 | 0.00% |
| 3 | T_Recipient | EBasisGroesse-EinheitET | 0.000 | 1.000 | 0.00% |
| 3 | T_Recipient | EBasisGroesseWert-ET | 0.000 | 1.000 | 0.00% |
| 3 | T_Recipient | EBasisLandET | 0.000 | 1.000 | 0.00% |
| 3 | T_Recipient | EBasisPLZET | 0.000 | 1.000 | 0.00% |
| 3 | T_Recipient | EBasisRhesusfaktor-ET | 0.000 | 1.000 | 0.00% |
| 3 | T_Recipient | EBasisZentrum-KontaktierungET | 0.000 | 1.000 | 0.00% |
| 3 | T_Recipient | EBasisZentrum-RegistrierungET | 0.000 | 1.000 | 0.00% |
| 3 | T_Recipient | EIdEmpfaengerNr-ETET | 0.000 | 1.000 | 0.00% |
| 3 | T_Donor_PM_Crossmatch | SPostmLaborCrossm-AuftragDateDSO | 0.000 | 1.000 | 0.00% |
| 3 | T_Donor_PM_Crossmatch | SPostmLaborCrossm-BefundDateDSO | 0.000 | 1.000 | 0.00% |
| 3 | T_Donor_PM_Crossmatch | SPostmLabor-CrossmEmpfaenger-IDpotentiellDSO | 0.000 | 1.000 | 0.00% |
| 3 | T_Donor_PM_Crossmatch | SPostmLaborCrossm-ErfahrenAmDateDSO | 0.000 | 1.000 | 0.00% |
| 3 | T_Donor_PM_Crossmatch | SPostmLaborCrossm-IdDSOKennnummerDSO | 0.000 | 1.000 | 0.00% |

| | | | | | |
|---|---|---|---|---|---|
| 3 | T_Donor_PM_Crossmatch | SPostmLaborCrossm-IdEmpfaengerNr-ETDSO | 0.000 | 1.000 | 0.00% |
| 3 | T_Donor_PM_Crossmatch | SPostmLaborCrossm-IdSpenderNrETDSO | 0.000 | 1.000 | 0.00% |
| 3 | T_Donor_PM_Crossmatch | SPostmLaborCrossm-LNRDSO | 0.000 | 1.000 | 0.00% |
| 3 | T_Donor_PM_Crossmatch | SPostmLaborCrossm-NRDSO | 0.000 | 1.000 | 0.00% |
| 3 | T_Donor_PM_Crossmatch | SPostmLaborCrossm-RangDSO | 0.000 | 1.000 | 0.00% |
| 3 | T_Donor_PM_Crossmatch | SPostmLaborCrossm-TXCETDSO | 0.000 | 1.000 | 0.00% |
| 3 | T_Donor_PM_Crossmatch | SPostmLaborCrossm-XMERGDSO | 0.000 | 1.000 | 0.00% |
| 3 | T_Donor_PM_Crossmatch | SPostmLaborCrossm-XMESPDSO | 0.077 | 0.907 | 8.40% |
| 3 | T_Donor_PM_Crossmatch | SPostmLaborCrossm-XMIGMDSO | 0.056 | 0.933 | 6.00% |
| 3 | T_Donor_PM_Crossmatch | SPostmLaborCrossm-XMREGDSO | 0.000 | 1.000 | 0.00% |
| 3 | T_Donor_PM_Crossmatch | SPostmLaborCrossm-XMSDateDSO | 0.079 | 0.883 | 9.40% |
| 3 | T_Donor_PM_Blood_Gas | SPostmLabor-BGErfahrenAmDate-DSO | 0.002 | 0.823 | 8.20% |
| 3 | T_Donor_PM_Blood_Gas | SPostmLaborBGId-DSOKennnummerDSO | 0.000 | 0.825 | 8.00% |
| 3 | T_Donor_PM_Blood_Gas | SPostmLaborBGId-SpenderNrETDSO | 0.000 | 0.825 | 8.00% |
| 3 | T_Donor_PM_Blood_Gas | SPostmLaborBGId-SpenderNrETET | 0.000 | 0.975 | 1.00% |
| 3 | T_Donor_PM_Blood_Gas | SPostmLaborBGProbe-DateDSO | 0.000 | 0.825 | 8.00% |
| 3 | T_Donor_PM_Blood_Gas | SPostmLaborBGProbe-DateET | 0.000 | 0.975 | 1.00% |
| 3 | T_Donor_PM_Monitor | SPostmMonit-Blutdruck-DiastolischEinheit-ET | 0.046 | 0.859 | 10.50% |

| | | | | | |
|---|---|---|---|---|---|
| 3 | T_Donor_PM_Monitor | SPostmMonit-Blutdruck-DiastolischWertET | 0.046 | 0.859 | 10.50% |
| 3 | T_Donor_PM_Monitor | SPostmMonit-BlutdruckSystolisch-EinheitET | 0.044 | 0.863 | 10.20% |
| 3 | T_Donor_PM_Monitor | SPostmMonit-BlutdruckSystolisch-WertET | 0.044 | 0.863 | 10.20% |
| 3 | T_Donor_PM_Monitor | SPostmMonitDateET | 0.000 | 0.983 | 1.10% |
| 3 | T_Donor_PM_Monitor | SPostmMonit-HfrequenzEinheitET | 0.056 | 0.842 | 11.90% |
| 3 | T_Donor_PM_Monitor | SPostmMonit-HfrequenzWertET | 0.056 | 0.842 | 11.90% |
| 3 | T_Donor_PM_Monitor | SPostmMonitId-SpenderNrETET | 0.000 | 0.983 | 1.10% |
| 3 | T_Donor_PM_Monitor | SPostmMonit-TemperaturEinheit-ET | 0.074 | 0.816 | 14.20% |
| 3 | T_Donor_PM_Monitor | SPostmMonit-TemperaturWertET | 0.074 | 0.816 | 14.20% |
| 3 | T_Donor_PM_Urine | SPostmLabor-URIErfahrenAmDate-DSO | 0.002 | 0.876 | 4.90% |
| 3 | T_Donor_PM_Urine | SPostmLabor-URIGlukoseDSO | 0.015 | 0.851 | 6.70% |
| 3 | T_Donor_PM_Urine | SPostmLaborURIId-DSOKennnummerDSO | 0.000 | 0.880 | 4.60% |
| 3 | T_Donor_PM_Urine | SPostmLaborURIId-SpenderNrETDSO | 0.000 | 0.880 | 4.60% |
| 3 | T_Donor_PM_Urine | SPostmLabor-URIProbeDateDSO | 0.000 | 0.880 | 4.60% |
| 3 | T_Donor_PM_Urine | SPostmLabor-URIProteinDSO | 0.011 | 0.858 | 6.10% |
| 3 | T_Donor_PM_Virology | SPostmLabor-VIRErfahrenAmDate-DSO | 0.001 | 0.796 | 12.30% |
| 3 | T_Donor_PM_Virology | SPostmLaborVIRId-DSOKennnummerDSO | 0.000 | 0.800 | 12.00% |
| 3 | T_Donor_PM_Virology | SPostmLaborVIRId-SpenderNrETDSO | 0.000 | 0.800 | 12.00% |

| | | | | | |
|---|---|---|---|---|---|
| 3 | T_Donor_PM_Virology | SPostmLaborVIRId-SpenderNrETET | 0.000 | 0.823 | 8.00% |
| 3 | T_Donor_PM_Virology | SPostmLabor-VIRProbeDateDSO | 0.000 | 0.800 | 12.00% |
| 3 | T_Donor_PM_Virology | SPostmLabor-VIRProbeDateET | 0.000 | 0.823 | 8.00% |
| 3 | T_Donor_PM | SPostmAnamn-AlkoholkonsumDSO | 0.009 | 0.756 | 12.60% |
| 3 | T_Donor_PM | SPostmAnamn-DrogenkonsumDSO | 0.016 | 0.749 | 13.20% |
| 3 | T_Donor_PM | SPostmAnamnRaucher-DSO | 0.009 | 0.755 | 12.60% |
| 3 | T_Donor_PM | SPostmAnamnRaucher-ET | 0.014 | 0.828 | 8.10% |
| 3 | T_Donor_PM | SPostmBasis-Abschaltung-LebenserhaltungDate-ET | 0.000 | 0.842 | 6.70% |
| 3 | T_Donor_PM | SPostmBasisAlter-DSO | 0.000 | 0.774 | 11.20% |
| 3 | T_Donor_PM | SPostmBasis-AufnahmeDateET | 0.000 | 0.842 | 6.70% |
| 3 | T_Donor_PM | SPostmBasis-BeatmungBeginnDate-ET | 0.001 | 0.842 | 6.80% |
| 3 | T_Donor_PM | SPostmBasisBlutgr-ET | 0.000 | 0.842 | 6.70% |
| 3 | T_Donor_PM | SPostmBasis-DSORegionDSO | 0.000 | 0.774 | 11.20% |
| 3 | T_Donor_PM | SPostmBasis-ExplantationDateET | 0.002 | 0.841 | 6.90% |
| 3 | T_Donor_PM | SPostmBasis-GeburtsdatumET | 0.000 | 0.842 | 6.70% |
| 3 | T_Donor_PM | SPostmBasis-GeschlechtDSO | 0.000 | 0.774 | 11.20% |
| 3 | T_Donor_PM | SPostmBasis-GeschlechtET | 0.000 | 0.842 | 6.70% |
| 3 | T_Donor_PM | SPostmBasisGewicht-EinheitDSO | 0.000 | 0.774 | 11.20% |
| 3 | T_Donor_PM | SPostmBasisGewicht-EinheitET | 0.000 | 0.842 | 6.70% |

| | | | | | |
|---|---|---|---|---|---|
| 3 | T_Donor_PM | SPostmBasisGewicht-WertDSO | 0.000 | 0.774 | 11.20% |
| 3 | T_Donor_PM | SPostmBasisGewicht-WertET | 0.000 | 0.842 | 6.70% |
| 3 | T_Donor_PM | SPostmBasisGroesse-EinheitDSO | 0.000 | 0.774 | 11.20% |
| 3 | T_Donor_PM | SPostmBasisGroesse-EinheitET | 0.000 | 0.842 | 6.70% |
| 3 | T_Donor_PM | SPostmBasisGroesse-WertDSO | 0.000 | 0.774 | 11.20% |
| 3 | T_Donor_PM | SPostmBasisGroesse-WertET | 0.000 | 0.842 | 6.70% |
| 3 | T_Donor_PM | SPostmBasis-HstillstandDauer-EinheitET | 0.000 | 0.842 | 6.70% |
| 3 | T_Donor_PM | SPostmBasis-HstillstandDauer-WertET | 0.000 | 0.842 | 6.70% |
| 3 | T_Donor_PM | SPostmBasis-HypotensiveEpisode-DauerEinheitET | 0.000 | 0.842 | 6.70% |
| 3 | T_Donor_PM | SPostmBasis-HypotensiveEpisode-DauerWertET | 0.000 | 0.842 | 6.70% |
| 3 | T_Donor_PM | SPostmBasis-Intensivbehandlung-BeginnDateET | 0.001 | 0.842 | 6.80% |
| 3 | T_Donor_PM | SPostmBasisMeldung-KHDSO | 0.000 | 0.774 | 11.20% |
| 3 | T_Donor_PM | SPostmBasisMeldung-KHOrtDSO | 0.000 | 0.774 | 11.20% |
| 3 | T_Donor_PM | SPostmBasisMeldung-ZeitpunktDSO | 0.000 | 0.774 | 11.20% |
| 3 | T_Donor_PM | SPostmBasisPostm-TypET | 0.000 | 0.842 | 6.70% |
| 3 | T_Donor_PM | SPostmBasis-Registrierungszeitpunkt-ETDSO | 0.007 | 0.763 | 12.10% |
| 3 | T_Donor_PM | SPostmBasis-RhesusfaktorET | 0.000 | 0.842 | 6.70% |

| | | | | | |
|---|---|---|---|---|---|
| 3 | T_Donor_PM | SPostmBasisSpender-AusAuslandDSO | 0.000 | 0.774 | 11.20% |
| 3 | T_Donor_PM | SPostmBasis-SpenderartET | 0.000 | 0.842 | 6.70% |
| 3 | T_Donor_PM | SPostmBasis-SpenderstatusDSO | 0.000 | 0.774 | 11.20% |
| 3 | T_Donor_PM | SPostmBasisStatus-DarmDSO | 0.003 | 0.770 | 11.60% |
| 3 | T_Donor_PM | SPostmBasisStatus-LesplitLinksDSO | 0.019 | 0.756 | 13.00% |
| 3 | T_Donor_PM | SPostmBasisStatus-LesplitRechtsDSO | 0.019 | 0.757 | 13.00% |
| 3 | T_Donor_PM | SPostmBasis-UrinkatheterBeginn-DateET | 0.009 | 0.835 | 7.60% |
| 3 | T_Donor_PM | SPostmBasis-ZeitpunktHirntodET | 0.000 | 0.842 | 6.70% |
| 3 | T_Donor_PM | SPostmId-DSOKennnummerDSO | 0.000 | 0.774 | 11.20% |
| 3 | T_Donor_PM | SPostmIdSpenderNr-ETDSO | 0.000 | 0.774 | 11.20% |
| 3 | T_Donor_PM | SPostmIdSpenderNr-ETET | 0.000 | 0.842 | 6.70% |
| 3 | T_Donor_PM | SPostmRechtl-EignungEntscheidung-DarmDSO | 0.000 | 0.774 | 11.20% |
| 3 | T_Donor_PM | SPostmRechtl-EignungEntscheidung-HDSO | 0.000 | 0.774 | 11.20% |
| 3 | T_Donor_PM | SPostmRechtl-EignungEntscheidung-LeDSO | 0.000 | 0.774 | 11.20% |
| 3 | T_Donor_PM | SPostmRechtl-EignungEntscheidung-LuLinksDSO | 0.000 | 0.774 | 11.20% |
| 3 | T_Donor_PM | SPostmRechtl-EignungEntscheidung-LuRechtsDSO | 0.000 | 0.774 | 11.20% |
| 3 | T_Donor_PM | SPostmRechtl-EignungEntscheidung-NLinksDSO | 0.000 | 0.774 | 11.20% |

| | | | | | |
|---|---|---|---|---|---|
| 3 | T_Donor_PM | SPostmRechtl-EignungEntscheidung-NRechtsDSO | 0.000 | 0.774 | 11.20% |
| 3 | T_Donor_PM | SPostmRechtl-EignungEntscheidung-PDSO | 0.000 | 0.774 | 11.20% |
| 3 | T_Donor_PM | SPostmRechtl-Eignung-Entscheidungszeitpunkt-DSO | 0.000 | 0.774 | 11.20% |
| 3 | T_Kidney_Retrieval | ONAnzahlArterien-DSO | 0.000 | 0.912 | 4.30% |
| 3 | T_Kidney_Retrieval | ONAnzahlArterienET | 0.001 | 0.974 | 0.40% |
| 3 | T_Kidney_Retrieval | ONAnzahlVenenDSO | 0.000 | 0.912 | 4.30% |
| 3 | T_Kidney_Retrieval | ONAnzahlVenenET | 0.001 | 0.973 | 0.40% |
| 3 | T_Kidney_Retrieval | ONArtLaengeUreter-DSO | 0.002 | 0.910 | 4.50% |
| 3 | T_Kidney_Retrieval | ONArteriePatchDSO | 0.002 | 0.911 | 4.40% |
| 3 | T_Kidney_Retrieval | ONArteriePatchET | 0.003 | 0.969 | 0.60% |
| 3 | T_Kidney_Retrieval | ONEnBlocEntnahme-DSO | 0.029 | 0.880 | 7.30% |
| 3 | T_Kidney_Retrieval | ONEntnahmeDateDSO | 0.000 | 0.914 | 4.20% |
| 3 | T_Kidney_Retrieval | ONEntnahmekrankenhaus-ET | 0.001 | 0.975 | 0.40% |
| 3 | T_Kidney_Retrieval | ONEntnahmezentrum-DSO | 0.000 | 0.914 | 4.20% |
| 3 | T_Kidney_Retrieval | ONHeparinDateET | 0.018 | 0.941 | 2.30% |
| 3 | T_Kidney_Retrieval | ONHeparinVolumen-EinheitET | 0.000 | 0.982 | 0.20% |
| 3 | T_Kidney_Retrieval | ONHeparinVolumen-WertET | 0.018 | 0.941 | 2.30% |
| 3 | T_Kidney_Retrieval | ONIdDSOKennnummer-DSO | 0.000 | 0.914 | 4.20% |
| 3 | T_Kidney_Retrieval | ONIdSpenderNr-ETDSO | 0.000 | 0.914 | 4.20% |
| 3 | T_Kidney_Retrieval | ONIdSpenderNrETET | 0.000 | 0.982 | 0.20% |
| 3 | T_Kidney_Retrieval | ONId-Transplantationsnummer-ETET | 0.000 | 0.982 | 0.20% |
| 3 | T_Kidney_Retrieval | ONIschaemiezeitWarm-ErsteEinheitET | 0.000 | 0.982 | 0.20% |

| | | | | | |
|---|---|---|---|---|---|
| 3 | T_Kidney_Retrieval | ONLaengeUreterET | 0.003 | 0.970 | 0.60% |
| 3 | T_Kidney_Retrieval | ONNephrektomieDate-ET | 0.001 | 0.976 | 0.30% |
| 3 | T_Kidney_Retrieval | ONOPZeiten-CrossclampDateDSO | 0.000 | 0.914 | 4.20% |
| 3 | T_Kidney_Retrieval | ONOPZeitenNahtDate-DSO | 0.000 | 0.914 | 4.20% |
| 3 | T_Kidney_Retrieval | ONOPZeitenSchnitt-DateDSO | 0.000 | 0.914 | 4.20% |
| 3 | T_Kidney_Retrieval | ONOrganTypDSO | 0.000 | 0.914 | 4.20% |
| 3 | T_Kidney_Retrieval | ONOrganTypET | 0.000 | 0.982 | 0.20% |
| 3 | T_Kidney_Retrieval | ONOrganqualitaetDSO | 0.004 | 0.908 | 4.70% |
| 3 | T_Kidney_Retrieval | ONOrganqualitaetET | 0.008 | 0.961 | 1.20% |
| 3 | T_Kidney_Retrieval | ONPerfusionKalt-StartDateET | 0.000 | 0.982 | 0.20% |
| 3 | T_Kidney_Retrieval | ONPerfusionLoesung-ET | 0.001 | 0.974 | 0.40% |
| 3 | T_Kidney_Retrieval | ONPerfusion-MaschinellDSO | 0.034 | 0.871 | 8.00% |
| 3 | T_Kidney_Retrieval | ONPerfusion-MaschinellET | 0.083 | 0.858 | 8.90% |
| 3 | T_Kidney_Retrieval | ONPerfusion-QualitaetDSO | 0.002 | 0.911 | 4.40% |
| 3 | T_Kidney_Retrieval | ONPerfusion-QualitaetET | 0.004 | 0.967 | 0.70% |
| 3 | T_Kidney_Retrieval | ONPerfusionVolumen-EinheitET | 0.000 | 0.982 | 0.20% |
| 3 | T_Kidney_Retrieval | ONPerfusionVolumen-WertET | 0.003 | 0.971 | 0.50% |
| 3 | T_Kidney_Retrieval | ONVenenPatchDSO | 0.005 | 0.909 | 4.70% |
| 3 | T_Kidney_Retrieval | ONVenenPatchET | 0.007 | 0.962 | 1.00% |
| 3 | T_Donor_PM_Tox | SPostmLabor-TOXErfahrenAmDate-DSO | 0.073 | 0.846 | 11.80% |
| 3 | T_Donor_PM_Tox | SPostmLaborTOXId-DSOKennnummerDSO | 0.000 | 1.000 | 0.00% |
| 3 | T_Donor_PM_Tox | SPostmLaborTOXId-SpenderNrETDSO | 0.000 | 1.000 | 0.00% |
| 3 | T_Donor_PM_Tox | SPostmLabor-TOXProbeDateDSO | 0.000 | 1.000 | 0.00% |

| | | | | | |
|---|---|---|---|---|---|
| 3 | T_Donor_PM_Tox | SPostmLabor-TOXProbenmaterial-DSO | 0.069 | 0.905 | 8.30% |
| 3 | T_Recip_Immuno | EImmAutoantikoerper-ET | 0.056 | 0.896 | 8.20% |
| 3 | T_Recip_Immuno | EImmDiagnostik-Screeningverfahren-ET | 0.056 | 0.896 | 8.20% |
| 3 | T_Recip_Immuno | EImmDiagnostik-ZentrumET | 0.000 | 1.000 | 0.00% |
| 3 | T_Recip_Immuno | EImmEingabeDateET | 0.000 | 1.000 | 0.00% |
| 3 | T_Recip_Immuno | EImmErgebnisTypET | 0.000 | 1.000 | 0.00% |
| 3 | T_Recip_Immuno | EImmIdEmpfaenger-NrETET | 0.000 | 1.000 | 0.00% |
| 3 | T_Recip_Immuno | EImmPRAEinheitET | 0.056 | 0.896 | 8.20% |
| 3 | T_Recip_Immuno | EImmPRAWertET | 0.056 | 0.896 | 8.20% |
| 3 | T_Recip_Immuno | EImmProbeDateET | 0.000 | 1.000 | 0.00% |
| 3 | T_Donor_PM_Diag | SPostmDiagnosen-Diagnose-BeschreibungDSO | 0.000 | 0.786 | 14.00% |
| 3 | T_Donor_PM_Diag | SPostmDiagnosen-DiagnoseICD10DSO | 0.000 | 0.786 | 14.00% |
| 3 | T_Donor_PM_Diag | SPostmDiagnosen-ErfahrenAmDateDSO | 0.000 | 0.786 | 14.00% |
| 3 | T_Donor_PM_Diag | SPostmDiagnosen-ErkrankungBeginn-DateDSO | 0.000 | 0.786 | 14.00% |
| 3 | T_Donor_PM_Diag | SPostmDiagnosenId-DSOKennnummerDSO | 0.000 | 0.786 | 14.00% |
| 3 | T_Donor_PM_Diag | SPostmDiagnosenId-SpenderNrETDSO | 0.000 | 0.786 | 14.00% |
| 3 | T_Donor_PM_Diag | SPostmDiagnosen-KlassifikationDSO | 0.000 | 0.786 | 14.00% |
| 4 | T_Recipient | EBasis-BluttransfusionVor-RegistrierungET | 0.332 | 0.567 | 35.60% |
| 4 | T_Recipient | EBasisNationalitaet-ET | 0.488 | 0.499 | 49.10% |
| 4 | T_Donor_PM_Crossmatch | SPostmLaborCrossm-XMBZDSO | 0.460 | 0.458 | 49.30% |

| | | | | | |
|---|---|---|---|---|---|
| 4 | T_Donor_PM_Crossmatch | SPostmLaborCrossm-XMIGGDSO | 0.584 | 0.391 | 59.40% |
| 4 | T_Donor_PM_Crossmatch | SPostmLaborCrossm-XMTZDSO | 0.434 | 0.498 | 46.10% |
| 4 | T_Kidney_Retrieval | ONAnzahlUreterDSO | 0.373 | 0.540 | 41.50% |

# 5 Supplementary Table 4

This table shows the results of the decision tree analysis. Only trees with any predictors are included, as postpruning might have removed all predictors.

Table 4

| Table (Data provider) | Test RMSE | Predictors |
|---|---|---|
| T_Kidney_Med (ET) | 0.000 | C_FNImmunsuppressionName |
| T_Recip_Immuno (ET) | 0.029 | C_EImmErgebnisTyp, C_EImm-DiagnostikZentrum |
| T_Donor_PM_Diag (DSO) | 0.033 | C_SPostmDiagnosenKlassifikation, C_SPostmDiagnosenHirnschaedigung-Art |
| T_Kidney_Retrieval (ET) | 0.047 | C_ONEntnahmekrankenhaus |
| T_Recip_Urgency (ET) | 0.055 | C_EDringlCode, C_EDringlOrgan |
| T_Donor_PM_Crossmatch (DSO) | 0.062 | C_SPostmLaborCrossmTXCET, C_SPostmLaborCrossmXMERG, C_SPostmLaborCrossmXMIGM |
| T_Transplantation (IQTIG) | 0.069 | C_TSpendeKompatibelNP, C_TKomplikationIntraPost-OperationAllgmeinNP, C_TPost-OPFunktionsaufnahmeTransplantatN |
| T_Donor_PM_Med (DSO) | 0.071 | C_SPostmMedienDosisEinheit, C_SPostmMedienApplikationsform |

| | | |
|---|---|---|
| T_Donor_PM (ET) | 0.076 | C_SPostmBasisHypotensive-EpisodeDauerWert, C_SPostm-BasisGewichtWert, C_SPostm-BasisGroesseWert, C_SPostmBasis-HstillstandDauerWert, C_SPostm-AnamnVorerkrankungenHypertonie, C_SPostmAnamnMalignitaet, C_SPostmBasisGeschlecht |
| T_Recipient (ET) | 0.078 | C_EBasisZentrumKontaktierung, C_EBasisZentrumRegistrierung, C_EBasisGeschlecht, C_EBasis-GroesseWert |
| T_Donor_PM (IQTIG) | 0.086 | C_SPostmBasisBeatmungDauerWert |
| T_Transplantation (ET) | 0.089 | C_TFollowUpZentrum, C_TTransplantationszentrum-Registrierung, C_TTransplantationszentrum, C_TDringl |
| T_Kidney_Retrieval (DSO) | 0.093 | C_ONEntnahmezentrum |
| T_Donor_PM_Blood_Gas (ET) | 0.098 | C_SPostmLaborBGpHO2100Prozent, C_SPostmLaborBGpO2O2100Prozent-Einheit, C_SPostmLaborBGp-O2Einheit, C_SPostmLabor-BGO2SaettigungO2100ProzentWert, C_SPostmLaborBGFiO2Wert, C_SPostmLaborBGPEEPWert, C_SPostmLaborBGBaseExcess-O2100ProzentWert, C_SPostmLabor-BGHCO3O2100ProzentWert, C_SPostm-LaborBGO2SaettigungWert |
| T_Donor_PM_Path (DSO) | 0.101 | C_SPostmLaborPATProbenmaterial |

| | | |
|---|---|---|
| T_Kidney_Followup (ET) | 0.102 | C_FNCenter, C_FNFollowUpArt, C_FNDialyse, C_FNHerkrankung-Koronar, C_FNHepatitis-Chronisch, C_FNDiabetes-Mellitus, C_FNHypertonie, C_FNKrankheitenAndere, C_FNTeilnahmeKlinischeStudie-ImmunsuppressiveMedikamente, C_FNInduktionstherapie, C_FNVerschlusskrankheitArteriell |
| T_Donor_PM_Monitor (ET) | 0.102 | C_SPostmMonitHstillstandDauer-Wert |
| T_Donor_PM_Blood_Type (DSO) | 0.115 | C_SPostmLaborBlutGr-Untersuchungsart |
| T_Kidney_Followup (IQTIG) | 0.119 | C_FNPatientVerstorben, C_FNGraftversagen, C_FNInstitutionskennzeichen |
| T_Donor_PM_Micro (DSO) | 0.120 | C_SPostmLaborMICERERG, C_SPostm-LaborMICProbenmaterial, C_SPostm- LaborMICKeimzahl |
| T_Donor_PM_HLA (DSO) | 0.128 | C_SPostmLaborHLADRDNA1, C_SPostmLaborHLADRBR1ET, C_SPostmLaborHLADQDNA1, C_SPostmLaborHLADQBR1ET, C_SPostmLaborHLAProbenmaterial, C_SPostmLaborHLADQDNA2, C_SPostmLaborHLADRSP1ET, C_SPostmLaborHLADRSP2ET |
| T_Donor_PM_Chem (DSO) | 0.130 | C_SPostmLabor-KCProbenmaterial, C_SPostm-LaborKCKalziumkonzentration-Wert, C_SPostmLabor-KCNatriumkonzentrationWert |
| T_Donor_PM_Urine (DSO) | 0.164 | C_SPostmLaborURIProtein, C_SPostmLaborURIBakterien, C_SPostmLaborURILeukozyten, C_SPostmLaborURIGlukose |

| | | |
|---|---|---|
| T_Donor_PM_Monitor (DSO) | 0.168 | C_SPostmMonitHstillstandDauer-Wert, C_SPostmMonitBlutdruck-SystolischWert, C_SPostmMonit-HypotensionDauerWert, C_SPostm-MonitBlutdruckDiastolischWert |
| T_Kidney_Waitlist (ET) | 0.181 | C_WNRegistrierungszentrum, C_WNGrunderkrankungBeschreibung, C_WNGrunderkrankung, C_WNGrunderkrankungBeschreibung-ICD10, C_WNGrunderkrankungICD10 |
| T_Donor_PM_Virology (DSO) | 0.185 | C_SPostmLaborVIRHBSAK, C_SPostm-LaborVIRProbenmaterial, C_SPostm- LaborVIRHBCAK, C_SPostmLabor- VIRCMVIgM, C_SPostmLabor-VIRToxoplasmose, C_SPostmLabor- VIRHIVAg |
| T_Donor_PM_Virology (ET) | 0.189 | C_SPostmLaborVIRMeningitis, C_SPostmLaborVIRSepsis, C_SPostmLaborVIRHBsAb, C_SPostmLaborVIRHIVAg, C_SPostm- LaborVIRLues, C_SPostmLabor- VIRHBcAb |
| T_Donor_PM_Tox (DSO) | 0.202 | C_SPostmLaborTOXAMS, C_SPostm- LaborTOXBDS, C_SPostmLabor- TOXBTS, C_SPostmLaborTOXOPS, C_SPostmLaborTOXABS, C_SPostm- LaborTOXADS |
| T_Donor_PM_Chem (ET) | 0.204 | C_SPostmLabor-KCNatriumkonzentration- Wert, C_SPostmLabor-KCKaliumkonzentrationWert |
| T_Donor_PM (DSO) | 0.239 | C_SPostmBasisDSORegion, C_SPostmAnamnAlkoholkonsum, C_SPostmAnamnRaucher |

## 6 Supplementary Figure 1-3

The number of subject types (recipients, donors, and transplantations) was counted by observing the total number of unique identifiers of each type across all tables from all data providers. The availability of data for each subject type was analyzed by counting the number of unique identifiers in each table. The co-occurrence of subjects together across tables was analyzed by counting the number of subject identifiers that occur together in groups of tables.

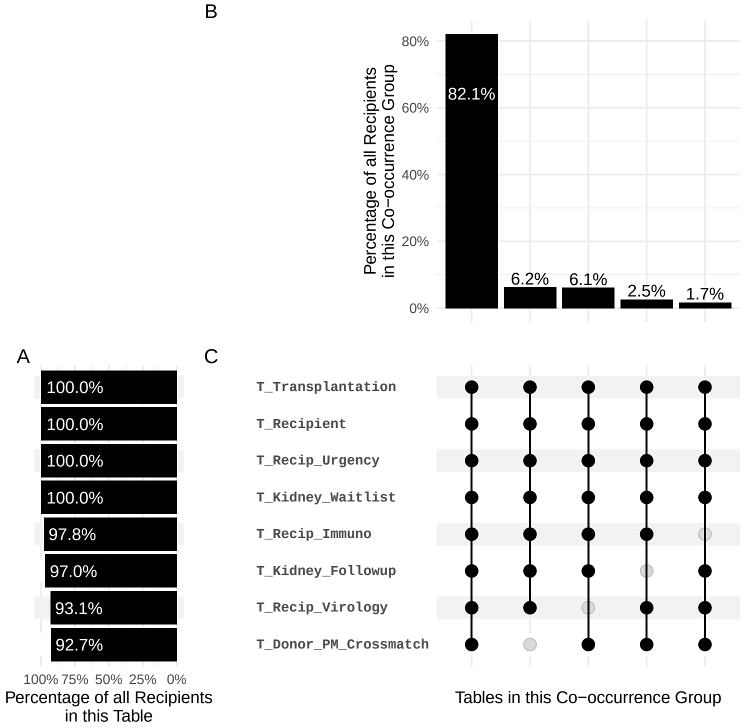


Figure 1: Recipient data availability and co-occurrence: In A the fraction of recipients with data in each table is shown. In B and C co-occurring groups of recipients are visualized. The different groups are visible on the x-axis. B shows the fraction of recipients referenced in each group, while C shows the tables which provide data for these recipients. For example, all recipients have data in the table `T_Transplantation` and the largest group of recipients is has data in all tables.

Data for 14,954 recipients are collected in 8 tables. To understand how much data is available for each recipient, we will look at the fraction of all recipients who have any data in each table. In Figure 1 A this availability is shown for each table with recipient data. All tables provide at least some data for 13,866 (93%) of all recipients. `T_Recipient`, `T_Recip_Urgency`, `T_Transplantation` and `T_Kidney_Waitlist` contain data for all recipients. However, data

in T_Recipient, T_Kidney_Waitlist and T_Transplantation was necessary for the creation of the target population. Thus, the availability of data in these tables was a selection criterion, leading to the 100% availability. To find groups of recipients, who occur in the same tables, co-occurrence of recipients was analyzed. These groups are relevant for the analysis and modeling tasks, where conditional availability needs to be accounted for. In Figure 1 B the number of recipients in each group are shown, while in Figure 1 C the tables in which these recipients occur are shown. For most recipients (12,271 (82%)) data is available in all tables. The remaining recipients have data available all tables except one.

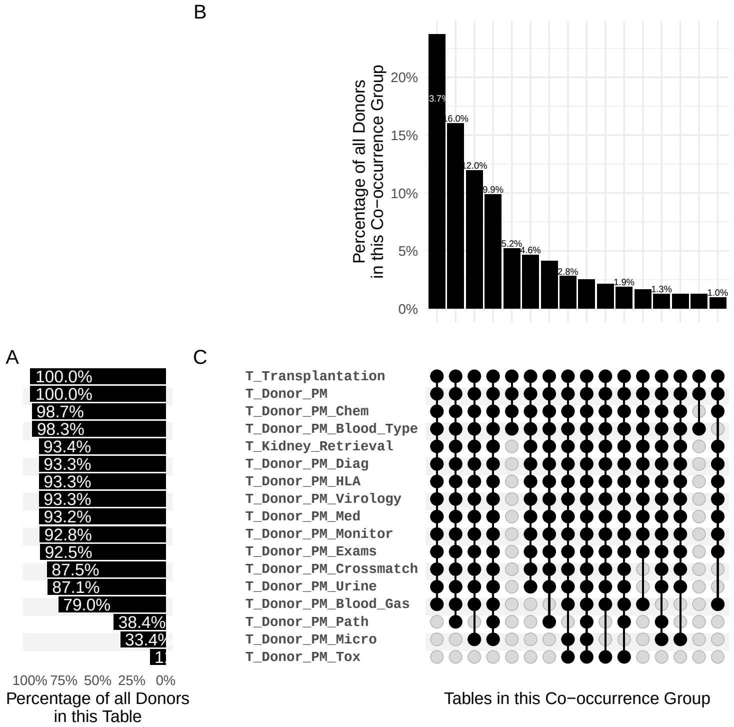


Figure 2: Donor data availability and co-occurrence: In A the fraction of donors with data in each table is shown. In B and C co-occurring groups of donors are visualized. The different groups are visible on the x-axis. B shows the fraction of donors referenced in each group, while C shows the tables which provide data for these donors. For example, all donors have data in the table Transplantation and the largest group of donors has data in all tables except Donor PM Path, Donor PM Micro and Donor PM Tox.

Data for 9,964 donors are collected in 17 tables. Data availability is shown in Figure 2 A. Of all donors 79% have at least some data in all tables except in T_Donor_PM_Path, T_Donor_PM_Micro and T_Donor_PM_Tox. These only contain data for 38%, 33% and 11%

of all donors respectively. T_Donor_PM and T_Transplantation contain data for all donors. This is due to the fact that availability in these tables was also necessary for the creation of the target population. The co-occurrence analysis for all occurence groups containing at least 1% of all donors is shown in Figure 2 B and C. Only 3% of all donors appear in all tables. 24% of donors appear in all tables except the three mentioned above. Most other donors appear in all tables except a few. Two groups visible in Figure 2 B and C are outliers. In these groups there are 5% and 1% of all donors respectively. The first group only occurs in T_Transplantation, T_Donor_PM, T_Donor_PM_Chem and T_Donor_PM_Blood_Type. The second group appears in the same tables except T_Donor_PM_Chem. These might be donors for which most data was not digitized or reported.

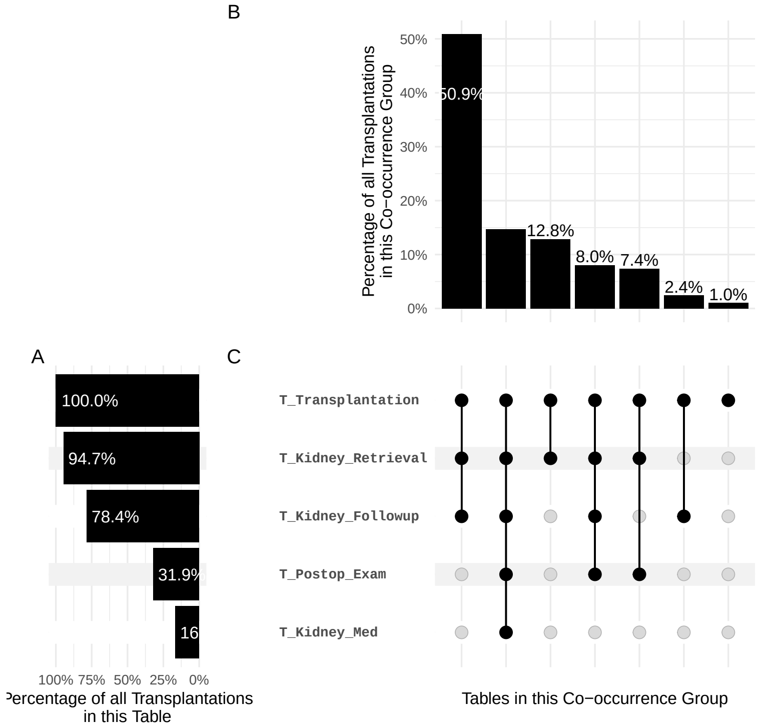


Figure 3: Transplantation data availability and co-occurrence: In A the fraction of transplantations with data in each table is shown. In B and C co-occurring groups of transplantations are visualized. The different groups are visible on the x-axis. B shows the fraction of transplantations referenced in each group, while C shows the tables which provide data for these transplantations. For example, all transplantations have data in the table Transplantation and the largest group of transplantations has data in the tables Transplantation, Kidney Retrieval and Kidney Followup.

Data for 14,954 transplantations are collected in 5 tables. Data availability is shown in Fig-

ure 3 A. Only Transplantation has data for all transplantations. Data in this table was again necessary for the creation of the target population. Follow-up data in T_Kidney_Followup is available for 78% of all transplantations. Only 32% and 17% of transplantations occur in T_Donor_PM_Exams and T_Kidney_Med. These might only have data when a post-operative examination or additional medication was necessary. Co-occurrence analysis for all groups containing at least 1% of all transplantations is shown in Figure 3 B and C. The largest group of transplantations representing 50.9% of all transplantations occurs in T_Transplantation, T_Kidney_Retrieval and T_Kidney_Followup. Transplantations are only referred to by ET. The other data providers use the recipient and donor together or alone to refer to the transplantations.

# 7 Supplementary Table 5

The following table shows which data provider contributed to which table.

Table 5

| Table | ET | IQTIG | DSO |
|---|---|---|---|
| T_Kidney_Med | Yes | No | No |
| T_Postop_Exam | Yes | No | No |
| T_Recip_Immuno | Yes | No | No |
| T_Recip_Urgency | Yes | No | No |
| T_Recip_Virology | Yes | No | No |
| T_Kidney_Followup | Yes | Yes | No |
| T_Kidney_Waitlist | Yes | Yes | No |
| T_Recipient | Yes | Yes | No |
| T_Transplantation | Yes | Yes | No |
| T_Donor_PM_Crossmatch | No | No | Yes |
| T_Donor_PM_Tox | No | No | Yes |
| T_Donor_PM_Blood_Gas | Yes | No | Yes |
| T_Donor_PM_Diag | Yes | No | Yes |
| T_Donor_PM_Exams | Yes | No | Yes |
| T_Donor_PM_HLA | Yes | No | Yes |
| T_Donor_PM_Med | Yes | No | Yes |
| T_Donor_PM_Micro | Yes | No | Yes |
| T_Donor_PM_Monitor | Yes | No | Yes |
| T_Donor_PM_Path | Yes | No | Yes |
| T_Donor_PM_Urine | Yes | No | Yes |
| T_Donor_PM_Virology | Yes | No | Yes |
| T_Donor_PM_Blood_Type | No | Yes | Yes |
| T_Donor_PM | Yes | Yes | Yes |
| T_Donor_PM_Chem | Yes | Yes | Yes |
| T_Kidney_Retrieval | Yes | Yes | Yes |

# 8 Supplementary Table 6-8

The following tables show whether the tables in the export contained long data or wide data. It is important to note, that there are sometimes columns which only have values for one of these observations, encoding wide data in the long format.

Table 6

| Table | Unique Rec. Count | Data provider | Avg. Rec. Observations |
|---|---|---|---|

| | | | |
|---|---|---|---|
| T_Kidney_Waitlist | 14954 | ET | 1.039655 |
| | | IQTIG | 1.002371 |
| T_Recip_Urgency | | ET | 4.194262 |
| T_Recipient | | ET | 1.000000 |
| | | IQTIG | 1.000000 |
| T_Transplantation | | ET | 1.000000 |
| | | IQTIG | 1.597549 |
| T_Recip_Immuno | 14629 | ET | 13.596760 |
| T_Kidney_Followup | 14499 | ET | 1.277436 |
| | | IQTIG | 2.564992 |
| T_Recip_Virology | 13915 | ET | 2.410061 |
| T_Donor_PM_Crossmatch | 13866 | DSO | 4.593033 |

Table 7

| Table | Unique Don. Count | Data provider | Avg. Don. Observations |
|---|---|---|---|
| T_Donor_PM | 9964 | DSO | 1.000000 |
| | | ET | 1.000000 |
| | | IQTIG | 1.000000 |
| T_Transplantation | | ET | 1.500803 |
| | | IQTIG | 1.648732 |
| T_Donor_PM_Chem | 9830 | DSO | 3.224760 |
| | | ET | 3.276774 |
| | | IQTIG | 1.460669 |
| T_Donor_PM_Blood_Type | 9796 | DSO | 2.465469 |
| | | IQTIG | 2.061320 |
| T_Kidney_Retrieval | 9311 | DSO | 1.535888 |
| | | ET | 1.520245 |
| | | IQTIG | 1.000000 |
| T_Donor_PM_Diag | 9300 | DSO | 6.449079 |
| | | ET | 1.000000 |
| T_Donor_PM_HLA | 9298 | DSO | 1.002716 |
| | | ET | 2.156264 |
| T_Donor_PM_Virology | 9297 | DSO | 1.386685 |
| | | ET | 1.381055 |
| T_Donor_PM_Med | 9288 | DSO | 9.100599 |
| | | ET | 4.068515 |

| | | | |
|---|---|---|---|
| T_Donor_PM_Monitor | 9249 | DSO<br>ET | 1.736944<br>1.868837 |
| T_Donor_PM_Exams | 9221 | DSO<br>ET | 4.518227<br>4.227865 |
| T_Donor_PM_Crossmatch | 8716 | DSO | 7.306907 |
| T_Donor_PM_Urine | 8675 | DSO<br>ET | 1.105066<br>1.052632 |
| T_Donor_PM_Blood_Gas | 7875 | DSO<br>ET | 2.197984<br>2.237478 |
| T_Donor_PM_Path | 3827 | DSO<br>ET | 1.467550<br>1.445739 |
| T_Donor_PM_Micro | 3332 | DSO<br>ET | 1.787917<br>3.046367 |
| T_Donor_PM_Tox | 1171 | DSO | 1.344150 |

Table 8

| Table | Unique Trans. Count | Data provider | Avg. Trans. Observations |
|---|---|---|---|
| T_Transplantation | 14954 | ET | 1.000000 |
| T_Kidney_Retrieval | 14155 | ET | 1.000000 |
| T_Kidney_Followup | 11718 | ET | 1.277436 |
| T_Postop_Exam | 4768 | ET | 5.800336 |
| T_Kidney_Med | 2471 | ET | 6.609875 |
